# Supplementary material for: Detecting Cohesive and 2-mode Communities in Directed and Undirected Networks
Source: arXiv:1401.7375 source file (2014-01-29)
Supplement: Supplementary file 1 [file 070appendix.tex]

\begin{itemize}
	\item ...
\end{itemize}
